# Supplementary material for: Generalizing Event-Based Motion Deblurring in Real-World Scenarios
Source: arXiv:2308.05932 source file (2023-08-11)
Supplement: Supplementary file 1 [file fig-msrbd.tex]

%子图大小

\begin{figure*}[t]
\centering
\begin{subfigure}{0.24\textwidth}
    \includegraphics[width=\linewidth]{imgs/supp/dataset/badminton.jpg}
    \caption*{Badminton}
\end{subfigure}
\begin{subfigure}{0.24\textwidth}
    \includegraphics[width=\linewidth]{imgs/supp/dataset/bag.jpg}
    \caption*{Bag}
\end{subfigure}
\begin{subfigure}{0.24\textwidth}
    \includegraphics[width=\linewidth]{imgs/supp/dataset/balls.jpg}
    \caption*{Balls}
\end{subfigure}
\begin{subfigure}{0.24\textwidth}
    \includegraphics[width=\linewidth]{imgs/supp/dataset/bike.jpg}
    \caption*{Bike}
\end{subfigure}
\\
\begin{subfigure}{0.24\textwidth}
    \includegraphics[width=\linewidth]{imgs/supp/dataset/book.jpg}
    \caption*{Book}
\end{subfigure}
\begin{subfigure}{0.24\textwidth}
    \includegraphics[width=\linewidth]{imgs/supp/dataset/book2.jpg}
    \caption*{Book2}
\end{subfigure}
\begin{subfigure}{0.24\textwidth}
    \includegraphics[width=\linewidth]{imgs/supp/dataset/building.jpg}
    \caption*{Building}
\end{subfigure}
\begin{subfigure}{0.24\textwidth}
    \includegraphics[width=\linewidth]{imgs/supp/dataset/card.jpg}
    \caption*{Card}
\end{subfigure}
\\
\begin{subfigure}{0.24\textwidth}
    \includegraphics[width=\linewidth]{imgs/supp/dataset/chessboard.jpg}
    \caption*{Chessboard}
\end{subfigure}
\begin{subfigure}{0.24\textwidth}
    \includegraphics[width=\linewidth]{imgs/supp/dataset/chinese.jpg}
    \caption*{Chinese}
\end{subfigure}
\begin{subfigure}{0.24\textwidth}
    \includegraphics[width=\linewidth]{imgs/supp/dataset/cube.jpg}
    \caption*{Cube}
\end{subfigure}
\begin{subfigure}{0.24\textwidth}
    \includegraphics[width=\linewidth]{imgs/supp/dataset/cylinders.jpg}
    \caption*{Cylinders}
\end{subfigure}
\\
\begin{subfigure}{0.24\textwidth}
    \includegraphics[width=\linewidth]{imgs/supp/dataset/desk.jpg}
    \caption*{Desk}
\end{subfigure}
\begin{subfigure}{0.24\textwidth}
    \includegraphics[width=\linewidth]{imgs/supp/dataset/dog.jpg}
    \caption*{Dog}
\end{subfigure}
\begin{subfigure}{0.24\textwidth}
    \includegraphics[width=\linewidth]{imgs/supp/dataset/english.jpg}
    \caption*{English}
\end{subfigure}
\begin{subfigure}{0.24\textwidth}
    \includegraphics[width=\linewidth]{imgs/supp/dataset/game.jpg}
    \caption*{Game}
\end{subfigure}
\\
\begin{subfigure}{0.24\textwidth}
    \includegraphics[width=\linewidth]{imgs/supp/dataset/game2.jpg}
    \caption*{Game2}
\end{subfigure}
\begin{subfigure}{0.24\textwidth}
    \includegraphics[width=\linewidth]{imgs/supp/dataset/mall.jpg}
    \caption*{Mall}
\end{subfigure}
\begin{subfigure}{0.24\textwidth}
    \includegraphics[width=\linewidth]{imgs/supp/dataset/poster.jpg}
    \caption*{Poster}
\end{subfigure}
\begin{subfigure}{0.24\textwidth}
    \includegraphics[width=\linewidth]{imgs/supp/dataset/printer.jpg}
    \caption*{Printer}
\end{subfigure}
\\
\begin{subfigure}{0.24\textwidth}
    \includegraphics[width=\linewidth]{imgs/supp/dataset/road.jpg}
    \caption*{Road}
\end{subfigure}
\begin{subfigure}{0.24\textwidth}
    \includegraphics[width=\linewidth]{imgs/supp/dataset/street.jpg}
    \caption*{Street}
\end{subfigure}
\begin{subfigure}{0.24\textwidth}
    \includegraphics[width=\linewidth]{imgs/supp/dataset/text.jpg}
    \caption*{Text}
\end{subfigure}
\begin{subfigure}{0.24\textwidth}
    \includegraphics[width=\linewidth]{imgs/supp/dataset/tools.jpg}
    \caption*{Tools}
\end{subfigure}
    % \vspace{-0.5em}
	\caption{Examples in our MS-RBD, where frames are at size 1152×768 and events are at size 288×192. The events accumulated over the exposure time of blurry frames are shown at the bottom right of the corresponding frames (red/blue dots denote positive/negative events). }
    \vspace{-1em}
	\label{fig:msrbd}
\end{figure*}
