# Supplementary material for: Generalizing Event-Based Motion Deblurring in Real-World Scenarios
Source: arXiv:2308.05932 source file (2023-08-11)
Supplement: Supplementary file 2 [file tab-msrbd.tex]

\begin{table*}[t]
\centering
% \small

\caption{Overview of our MS-RBD. \#Event indicates the total number of events in the sequence. FPS is the frame rate of the FLIR camera. Dynamic/Static shows whether the target scene is dynamic or static. }
\begin{tabular}{c|cccccc}
% \hline \hline
\toprule[2pt]
\textbf{Scene}            & \textbf{Sequence} & \textbf{Train/Test} & \textbf{\#Event (K)} & \textbf{FPS} & \textbf{Dynamic/Static} & \textbf{Camera Motion} \\ \midrule[1pt]
\multirow{22}{*}{Indoor}  & Badminton         & Train               & 8096                 & 15           & Static         & Rotation               \\
                          & Book              & Train               & 12128                & 15           & Static         & Rotation               \\
                          & Book2             & Train               & 3647                 & 15           & Dynamic        & No motion              \\
                          & Card              & Train               & 3351                 & 15           & Dynamic        & No motion              \\
                          & Chinese           & Train               & 13584                & 15           & Dynamic        & No motion              \\
                          & Cube              & Train               & 2026                 & 15           & Dynamic        & No motion              \\
                          & Cube2             & Train               & 6114                 & 15           & Dynamic        & No motion              \\
                          & Cylinders         & Train               & 9119                 & 15           & Static         & Rotation               \\
                          & Cylinders2        & Train               & 11389                & 15           & Static         & Random                 \\
                          & Desk              & Train               & 7703                 & 15           & Static         & Rotation               \\
                          & English           & Train               & 6582                 & 15           & Dynamic        & No motion              \\
                          & Game2             & Train               & 7751                 & 15           & Static         & Rotation               \\
                          & Printer           & Train               & 6312                 & 15           & Static         & Rotation               \\
                          & Printer2          & Train               & 8809                 & 15           & Static         & Random                 \\
                          & Tools             & Train               & 7193                 & 15           & Static         & Rotation               \\
                          & Toys              & Train               & 4765                 & 15           & Static         & Rotation               \\
                          & Toys2             & Train               & 6422                 & 15           & Static         & Random                 \\
                          & Bag               & Test                & 9892                 & 15           & Dynamic        & No motion              \\
                          & Balls             & Test                & 5182                 & 15           & Static         & Rotation               \\
                          & Balls2            & Test                & 5622                 & 15           & Static         & Random                 \\
                          & Chessboard        & Test                & 5574                 & 15           & Dynamic        & No motion              \\
                          & Game              & Test                & 7075                 & 15           & Static         & Random                 \\ \midrule[1pt]
\multirow{10}{*}{Outdoor} & Bike              & Train               & 6810                 & 30           & Static         & Random                 \\
                          & Poster            & Train               & 1328                 & 30           & Static         & Rotation               \\
                          & Poster2           & Train               & 3070                 & 15           & Static         & Random                 \\
                          & Road              & Train               & 2732                 & 15           & Dynamic        & Rotation               \\
                          & Road2             & Train               & 2888                 & 15           & Dynamic        & Rotation               \\
                          & Street            & Train               & 3198                 & 30           & Dynamic        & Random                 \\
                          & Text              & Train               & 1158                 & 15           & Static         & Rotation               \\
                          & Building          & Test                & 3066                 & 15           & Static         & Rotation               \\
                          & Dog               & Test                & 2026                 & 15           & Static         & Rotation               \\
                          & Mall              & Test                & 4403                 & 30           & Static         & Random                 \\ \bottomrule[2pt] %\hline \hline
\end{tabular}
\label{tab:msrbd}
\end{table*}
