# Supplementary material for: Generalizing Event-Based Motion Deblurring in Real-World Scenarios
Source: arXiv:2308.05932 source file (2023-08-11)
Supplement: Supplementary file 3 [file fig-add-res.tex]

\def\imgWidth{0.195\textwidth} %子图大小

\def\ssizz{1cm} %框大小
\def\ssmag{3}

% ev-reds
\def\sccevreds{(-1.65,-0.7)}
\def\smallboxlocevreds{(1.05,-0.45)} % 绿色小方框位置
\def\largeboxlocevreds{(-0.65, 0.3)} % 绿色大方框位置

% hs-ergb
\def\scchsergb{(-1.65,-1.35)}
\def\smallboxlochsergb{(0.35,-0.55)} % 绿色小方框位置
\def\largeboxlochsergb{(-0.65, 0.95)} % 绿色大方框位置

% ms-rbd
\def\scc{(-1.65,-0.96)}
\def\smallboxloc{(-0.7,-0.6)} % 绿色小方框位置
\def\smallboxlocout{(1.35,0.35)} % 绿色小方框位置
\def\largeboxloc{(-0.65, 0.59)} % 绿色大方框位置

\begin{figure*}[t]
	\centering
% EV-REDS -------------------------------
\tikzstyle{img} = [rectangle, minimum width=\imgWidth, draw=white]
	\begin{tikzpicture}	[spy using outlines={green,magnification=\ssmag,size=\ssizz},inner sep=0]
        \node [align=center, img] {\includegraphics[width=\imgWidth]{imgs/supp/additional/Ev-REDS/blur-1x.png}};
        \spy on \smallboxlocevreds in node [left] at \largeboxlocevreds;
        \node [anchor=west,font=\fontsize{8}{8}\selectfont] at \sccevreds {\textcolor{white}{\bf LR blur}};
	\end{tikzpicture}
	\begin{tikzpicture}	[spy using outlines={green,magnification=\ssmag,size=\ssizz},inner sep=0]
        \node [align=center, img] {\includegraphics[width=\imgWidth]{imgs/supp/additional/Ev-REDS/GT-1x.png}};
        \spy on \smallboxlocevreds in node [left] at \largeboxlocevreds;
        \node [anchor=west,font=\fontsize{8}{8}\selectfont] at \sccevreds {\textcolor{white}{\bf LR GT}};
	\end{tikzpicture}
	\begin{tikzpicture}	[spy using outlines={green,magnification=\ssmag,size=\ssizz},inner sep=0]
        \node [align=center, img] {\includegraphics[width=\imgWidth]{imgs/supp/additional/Ev-REDS/Motion-ETR-1x.png}};
        \spy on \smallboxlocevreds in node [left] at \largeboxlocevreds;
        \node [anchor=west,font=\fontsize{8}{8}\selectfont] at \sccevreds {\textcolor{white}{\bf Motion-ETR}};
	\end{tikzpicture}
	\begin{tikzpicture}	[spy using outlines={green,magnification=\ssmag,size=\ssizz},inner sep=0]
        \node [align=center, img] {\includegraphics[width=\imgWidth]{imgs/supp/additional/Ev-REDS/EVDI-1x.png}};
        \spy on \smallboxlocevreds in node [left] at \largeboxlocevreds;
        \node [anchor=west,font=\fontsize{8}{8}\selectfont] at \sccevreds {\textcolor{white}{\bf EVDI}};
	\end{tikzpicture}
	\begin{tikzpicture}	[spy using outlines={green,magnification=\ssmag,size=\ssizz},inner sep=0]
        \node [align=center, img] {\includegraphics[width=\imgWidth]{imgs/supp/additional/Ev-REDS/ours-1x.png}};
        \spy on \smallboxlocevreds in node [left] at \largeboxlocevreds;
        \node [anchor=west,font=\fontsize{8}{8}\selectfont] at \sccevreds {\textcolor{white}{\bf Ours}};
	\end{tikzpicture}
\\
\begin{tikzpicture}	[spy using outlines={green,magnification=\ssmag,size=\ssizz},inner sep=0]
        \node [align=center, img] {\includegraphics[width=\imgWidth]{imgs/supp/additional/Ev-REDS/blur-4x.png}};
        \spy on \smallboxlocevreds in node [left] at \largeboxlocevreds;
        \node [anchor=west,font=\fontsize{8}{8}\selectfont] at \sccevreds {\textcolor{white}{\bf HR blur}};
	\end{tikzpicture}
	\begin{tikzpicture}	[spy using outlines={green,magnification=\ssmag,size=\ssizz},inner sep=0]
        \node [align=center, img] {\includegraphics[width=\imgWidth]{imgs/supp/additional/Ev-REDS/GT-4x.png}};
        \spy on \smallboxlocevreds in node [left] at \largeboxlocevreds;
        \node [anchor=west,font=\fontsize{8}{8}\selectfont] at \sccevreds {\textcolor{white}{\bf HR GT}};
	\end{tikzpicture}
	\begin{tikzpicture}	[spy using outlines={green,magnification=\ssmag,size=\ssizz},inner sep=0]
        \node [align=center, img] {\includegraphics[width=\imgWidth]{imgs/supp/additional/Ev-REDS/Motion-ETR-4x.png}};
        \spy on \smallboxlocevreds in node [left] at \largeboxlocevreds;
        \node [anchor=west,font=\fontsize{8}{8}\selectfont] at \sccevreds {\textcolor{white}{\bf Motion-ETR}};
	\end{tikzpicture}
	\begin{tikzpicture}	[spy using outlines={green,magnification=\ssmag,size=\ssizz},inner sep=0]
        \node [align=center, img] {\includegraphics[width=\imgWidth]{imgs/supp/additional/Ev-REDS/EVDI+DASR-4x.png}};
        \spy on \smallboxlocevreds in node [left] at \largeboxlocevreds;
        \node [anchor=west,font=\fontsize{8}{8}\selectfont] at \sccevreds {\textcolor{white}{\bf EVDI+DASR}};
	\end{tikzpicture}
	\begin{tikzpicture}	[spy using outlines={green,magnification=\ssmag,size=\ssizz},inner sep=0]
        \node [align=center, img] {\includegraphics[width=\imgWidth]{imgs/supp/additional/Ev-REDS/Ours-4x.png}};
        \spy on \smallboxlocevreds in node [left] at \largeboxlocevreds;
        \node [anchor=west,font=\fontsize{8}{8}\selectfont] at \sccevreds {\textcolor{white}{\bf Ours}};
	\end{tikzpicture}

% HS-ERGB -------------------------------
\tikzstyle{img} = [rectangle, minimum width=\imgWidth, draw=white]
	\begin{tikzpicture}	[spy using outlines={green,magnification=\ssmag,size=\ssizz},inner sep=0]
        \node [align=center, img] {\includegraphics[width=\imgWidth]{imgs/supp/additional/HS-ERGB/blur-7.png}};
        \spy on \smallboxlochsergb in node [left] at \largeboxlochsergb;
        \node [anchor=west,font=\fontsize{8}{8}\selectfont] at \scchsergb {\textcolor{white}{\bf Normal blur}};
	\end{tikzpicture}
	\begin{tikzpicture}	[spy using outlines={green,magnification=\ssmag,size=\ssizz},inner sep=0]
        \node [align=center, img] {\includegraphics[width=\imgWidth]{imgs/supp/additional/HS-ERGB/GT-7.png}};
        \spy on \smallboxlochsergb in node [left] at \largeboxlochsergb;
        \node [anchor=west,font=\fontsize{8}{8}\selectfont] at \scchsergb {\textcolor{white}{\bf GT}};
	\end{tikzpicture}
	\begin{tikzpicture}	[spy using outlines={green,magnification=\ssmag,size=\ssizz},inner sep=0]
        \node [align=center, img] {\includegraphics[width=\imgWidth]{imgs/supp/additional/HS-ERGB/Motion-ETR-7.png}};
        \spy on \smallboxlochsergb in node [left] at \largeboxlochsergb;
        \node [anchor=west,font=\fontsize{8}{8}\selectfont] at \scchsergb {\textcolor{white}{\bf Motion-ETR}};
	\end{tikzpicture}
	\begin{tikzpicture}	[spy using outlines={green,magnification=\ssmag,size=\ssizz},inner sep=0]
        \node [align=center, img] {\includegraphics[width=\imgWidth]{imgs/supp/additional/HS-ERGB/EVDI-7.png}};
        \spy on \smallboxlochsergb in node [left] at \largeboxlochsergb;
        \node [anchor=west,font=\fontsize{8}{8}\selectfont] at \scchsergb {\textcolor{white}{\bf EVDI}};
	\end{tikzpicture}
	\begin{tikzpicture}	[spy using outlines={green,magnification=\ssmag,size=\ssizz},inner sep=0]
        \node [align=center, img] {\includegraphics[width=\imgWidth]{imgs/supp/additional/HS-ERGB/ours-7.png}};
        \spy on \smallboxlochsergb in node [left] at \largeboxlochsergb;
        \node [anchor=west,font=\fontsize{8}{8}\selectfont] at \scchsergb {\textcolor{white}{\bf Ours}};
	\end{tikzpicture}
\\
\begin{tikzpicture}	[spy using outlines={green,magnification=\ssmag,size=\ssizz},inner sep=0]
        \node [align=center, img] {\includegraphics[width=\imgWidth]{imgs/supp/additional/HS-ERGB/blur-13.png}};
        \spy on \smallboxlochsergb in node [left] at \largeboxlochsergb;
        \node [anchor=west,font=\fontsize{8}{8}\selectfont] at \scchsergb {\textcolor{white}{\bf Large blur}};
	\end{tikzpicture}
	\begin{tikzpicture}	[spy using outlines={green,magnification=\ssmag,size=\ssizz},inner sep=0]
        \node [align=center, img] {\includegraphics[width=\imgWidth]{imgs/supp/additional/HS-ERGB/GT-13.png}};
        \spy on \smallboxlochsergb in node [left] at \largeboxlochsergb;
        \node [anchor=west,font=\fontsize{8}{8}\selectfont] at \scchsergb {\textcolor{white}{\bf GT}};
	\end{tikzpicture}
	\begin{tikzpicture}	[spy using outlines={green,magnification=\ssmag,size=\ssizz},inner sep=0]
        \node [align=center, img] {\includegraphics[width=\imgWidth]{imgs/supp/additional/HS-ERGB/Motion-ETR-13.png}};
        \spy on \smallboxlochsergb in node [left] at \largeboxlochsergb;
        \node [anchor=west,font=\fontsize{8}{8}\selectfont] at \scchsergb {\textcolor{white}{\bf Motion-ETR}};
	\end{tikzpicture}
	\begin{tikzpicture}	[spy using outlines={green,magnification=\ssmag,size=\ssizz},inner sep=0]
        \node [align=center, img] {\includegraphics[width=\imgWidth]{imgs/supp/additional/HS-ERGB/EVDI-13.png}};
        \spy on \smallboxlochsergb in node [left] at \largeboxlochsergb;
        \node [anchor=west,font=\fontsize{8}{8}\selectfont] at \scchsergb {\textcolor{white}{\bf EVDI}};
	\end{tikzpicture}
	\begin{tikzpicture}	[spy using outlines={green,magnification=\ssmag,size=\ssizz},inner sep=0]
        \node [align=center, img] {\includegraphics[width=\imgWidth]{imgs/supp/additional/HS-ERGB/ours-13.png}};
        \spy on \smallboxlochsergb in node [left] at \largeboxlochsergb;
        \node [anchor=west,font=\fontsize{8}{8}\selectfont] at \scchsergb {\textcolor{white}{\bf Ours}};
	\end{tikzpicture}

%% ms-rbd ------------------------
 
	\tikzstyle{img} = [rectangle, minimum width=\imgWidth, draw=white]
	\begin{tikzpicture}	[spy using outlines={green,magnification=\ssmag,size=\ssizz},inner sep=0]
        \node [align=center, img] {\includegraphics[width=\imgWidth]{imgs/supp/additional/MS-RBD/Blur-in.png}};
        \spy on \smallboxloc in node [left] at \largeboxloc;
        \node [anchor=west,font=\fontsize{8}{8}\selectfont] at \scc {\textcolor{white}{\bf Blur}};
	\end{tikzpicture}
	\begin{tikzpicture}	[spy using outlines={green,magnification=\ssmag,size=\ssizz},inner sep=0]
        \node [align=center, img] {\includegraphics[width=\imgWidth]{imgs/supp/additional/MS-RBD/LEVS-in.png}};
        \spy on \smallboxloc in node [left] at \largeboxloc;
        \node [anchor=west,font=\fontsize{8}{8}\selectfont] at \scc {\textcolor{white}{\bf LEVS}};
	\end{tikzpicture}
	\begin{tikzpicture}	[spy using outlines={green,magnification=\ssmag,size=\ssizz},inner sep=0]
        \node [align=center, img] {\includegraphics[width=\imgWidth]{imgs/supp/additional/MS-RBD/Motion-ETR-in.png}};
        \spy on \smallboxloc in node [left] at \largeboxloc;
        \node [anchor=west,font=\fontsize{8}{8}\selectfont] at \scc {\textcolor{white}{\bf Motion-ETR}};
	\end{tikzpicture}
	\begin{tikzpicture}	[spy using outlines={green,magnification=\ssmag,size=\ssizz},inner sep=0]
        \node [align=center, img] {\includegraphics[width=\imgWidth]{imgs/supp/additional/MS-RBD/EVDI+DASR-in.png}};
        \spy on \smallboxloc in node [left] at \largeboxloc;
        \node [anchor=west,font=\fontsize{8}{8}\selectfont] at \scc {\textcolor{white}{\bf EVDI+DASR}};
	\end{tikzpicture}
	\begin{tikzpicture}	[spy using outlines={green,magnification=\ssmag,size=\ssizz},inner sep=0]
        \node [align=center, img] {\includegraphics[width=\imgWidth]{imgs/supp/additional/MS-RBD/Ours-in.png}};
        \spy on \smallboxloc in node [left] at \largeboxloc;
        \node [anchor=west,font=\fontsize{8}{8}\selectfont] at \scc {\textcolor{white}{\bf Ours}};
	\end{tikzpicture}
\\
\begin{tikzpicture}	[spy using outlines={green,magnification=\ssmag,size=\ssizz},inner sep=0]
        \node [align=center, img] {\includegraphics[width=\imgWidth]{imgs/supp/additional/MS-RBD/Blur-out.png}};
        \spy on \smallboxlocout in node [left] at \largeboxloc;
        \node [anchor=west,font=\fontsize{8}{8}\selectfont] at \scc {\textcolor{white}{\bf Blur}};
	\end{tikzpicture}
	\begin{tikzpicture}	[spy using outlines={green,magnification=\ssmag,size=\ssizz},inner sep=0]
        \node [align=center, img] {\includegraphics[width=\imgWidth]{imgs/supp/additional/MS-RBD/LEVS-out.png}};
        \spy on \smallboxlocout in node [left] at \largeboxloc;
        \node [anchor=west,font=\fontsize{8}{8}\selectfont] at \scc {\textcolor{white}{\bf LEVS}};
	\end{tikzpicture}
	\begin{tikzpicture}	[spy using outlines={green,magnification=\ssmag,size=\ssizz},inner sep=0]
        \node [align=center, img] {\includegraphics[width=\imgWidth]{imgs/supp/additional/MS-RBD/Motion-ETR-out.png}};
        \spy on \smallboxlocout in node [left] at \largeboxloc;
        \node [anchor=west,font=\fontsize{8}{8}\selectfont] at \scc {\textcolor{white}{\bf Motion-ETR}};
	\end{tikzpicture}
	\begin{tikzpicture}	[spy using outlines={green,magnification=\ssmag,size=\ssizz},inner sep=0]
        \node [align=center, img] {\includegraphics[width=\imgWidth]{imgs/supp/additional/MS-RBD/EVDI+DASR-out.png}};
        \spy on \smallboxlocout in node [left] at \largeboxloc;
        \node [anchor=west,font=\fontsize{8}{8}\selectfont] at \scc {\textcolor{white}{\bf EVDI+DASR}};
	\end{tikzpicture}
	\begin{tikzpicture}	[spy using outlines={green,magnification=\ssmag,size=\ssizz},inner sep=0]
        \node [align=center, img] {\includegraphics[width=\imgWidth]{imgs/supp/additional/MS-RBD/ours-out.png}};
        \spy on \smallboxlocout in node [left] at \largeboxloc;
        \node [anchor=west,font=\fontsize{8}{8}\selectfont] at \scc {\textcolor{white}{\bf Ours}};
	\end{tikzpicture}

	% \vspace{-0.75em}
	\caption{ Additional qualitative results on Ev-REDS (row 1-2), HS-ERGB (row 3-4), and MS-RBD (row 5-6).
 % Details are zoomed in for a better view.
	}
        % \vspace{-0.75em}
	\label{fig:add-res}
\end{figure*}
