# Supplementary material for: Generalizing Event-Based Motion Deblurring in Real-World Scenarios
Source: arXiv:2308.05932 source file (2023-08-11)
Supplement: Supplementary file 4 [file fig-net-details.tex]

\begin{figure}[t]
	\centering
	\includegraphics[width=\linewidth]{imgs/supp/fig-net-details.jpg}
	\caption{ Detailed architecture of our scale-aware network, where MSFF 16, 32, 64, and 128 indicate the MSFF block composed of a 4-layer MLP and a 1-layer DCN with the channel set to  16, 32, 64, and 128, respectively. }
	\label{fig:net-details}
\end{figure}
