# Supplementary material for: Generalizing Event-Based Motion Deblurring in Real-World Scenarios
Source: arXiv:2308.05932 source file (2023-08-11)
Supplement: Supplementary file 5 [file fig-setup.tex]

\begin{figure}[t]
	\centering
	\includegraphics[width=\linewidth]{imgs/supp/fig-setup.jpg}
	\caption{Illustration of our capture system, which is implemented with a beam splitter connecting a DAVIS346 event camera and a FLIR BlackFly S RGB camera. The system is mounted on a stabilizer to control the camera motion. }
	\label{fig:setup}
\end{figure}
