# Supplementary material for: Generalizing Event-Based Motion Deblurring in Real-World Scenarios
Source: arXiv:2308.05932 source file (2023-08-11)
Supplement: Supplementary file 7 [file tab-efficiency.tex]

\begin{table}[t]
\centering

\caption{Efficiency comparisons on the FLOPs required to infer a 160 × 320 image and the training hours needed on the Ev-REDS dataset. Best results are \textbf{bolded}. }
\begin{tabular}{lcc}
\toprule[2pt]
Method & FLOPs   & Training time \\ \midrule[1pt]
EVDI \cite{zhang2022unifying}   & 13.45 G & 48 hr         \\
Ours   & \textbf{11.15 G} & \textbf{22 hr}         \\ \bottomrule[2pt]
\end{tabular}
\label{tab:efficiency}
\end{table}
